# Supplementary material for: Evaluating Data-driven Performances of Mixed Integer Bilinear Formulations for Book Placement Planning
Source: arXiv:2406.04616 source file (2024-06-07)
Supplement: Supplementary file 1 [file sect_appendix.tex]

We explain the formulation that is used to solve the MIPs in Sec.~\ref{Sec:experiment_setup}.

For a non-convex constraint, we segment it into multiple regions and locally approximate or relax them into convex constraints. In this paper, we relax the bilinear constraints locally into convex polytopes (McCormick envelopes). Each polytope is associated with a unique combination of integer variable values, hence, mixed-integer convex constraints. Assume the number of regions used is $N$. Depending on the number of integer variables used, the formulation can generally be divided into 2 categories: 1) If the number of integer variables is $N$, we call it \textit{$N$ formulation}, e.g., the convex hull formulation \cite{belotti2011disjunctive}. 2) If the number of integer variables is $log_{2}N$, we call it \textit{$log_{2}N$ formulation}, e.g., \cite{vielma2011modeling}. \cite{vielma2011modeling} presents a \textit{$log_{2}N$ formulation} to model the special ordered sets of type 2 (sos2). However, there are several limitations of this formulation. For example, the segmented regions need to be connected to be a valid sos2 constraint, i.e., the two consecutive couple of non-zero entries can be any consecutive couple in the set. In this paper, we use MIP to model convex polytopes of arbitrary locations. This can increase the complexity for sos2 techniques as the polytopes can be disjunctive. The disjunctive constraints can be handled with convex hull formulations at a price of introducing more integer variables which may result in slower solving speeds.
% change difficulty to complexity--two sentences above

In this appendix, we demonstrate an intuitive but general \textit{$log_{2}N$ formulation} to model combinations of convex polytopes at any locations which serves as the base MIP formulation for the bilinear constraints in our paper. Assume the variable $\textbf{x}$ is enforced to be within one of the $N$ convex polytopes, denoted by $\textbf{A}_{i}\textbf{x} \leq \textbf{b}_{i}$, $i=1,...,N$. We introduce $m=log_{2}N$ binary variables $z_{1}, ..., z_{m}$, $z_{i} \in \{0,1\}$. Each combination of unique values of binary variables can be assigned to a convex polytope. Let the assignment be:
% Assume or we just assign them as such then simplify

\begin{equation}
    \textbf{z}=\Bar{\textbf{z}}_{i} \Rightarrow \textbf{A}_{i}\textbf{x} \leq \textbf{b}_{i}
\end{equation}

Where $\Bar{\textbf{z}}_{i} = [\Bar{z}_{i,1}, ..., \Bar{z}_{i,m}]$ are constant binary values associated with polytope $i$. Note $\Bar{z}_{i} \neq \Bar{z}_{j}$ if $i \neq j$. In other words, we require that when $\textbf{z}=\Bar{\textbf{z}}_{i}$, $\textbf{x}$ stays within the polytope $\textbf{A}_{i}\textbf{x} \leq \textbf{b}_{i}$; otherwise, the constraint is unenforced.

Denote the vertices of the polytopes by $\textbf{v}_{i,1}, ..., \textbf{v}_{i,n_{i}}$, $i=1, ..., N$, where $n_{i}$ is the number of vertices associated with polytope $i$. Each vertex $\textbf{v}_{i,j}$ is assigned a continuous non-negative variable $\lambda_{i,j} \in [0, 1]$. In general, one can run a mathematical program (e.g. \cite{avis1992pivoting}) to get vertices from the nondegenerate system of inequalities $\textbf{A}_{i}\textbf{x} \leq \textbf{b}_{i}$. As a result, the assignment becomes: 

\begin{equation}
    \textbf{z}=\Bar{\textbf{z}}_{i} \Rightarrow \ \ 
\begin{aligned}
    & \textbf{x} = \sum_{j=1}^{n_{i}} \lambda_{i,j} \textbf{v}_{i,j} \\
    & \sum_{j=1}^{n_{i}} \lambda_{i,j} = 1, \ \ \lambda_{i,j} \in [0, 1]
\end{aligned}
\label{Eqn:MICP_formulation_one}
\end{equation}

The formulation can be written as:

\begin{equation}
\begin{aligned}
    & (5.a) \quad \textbf{x} = \sum_{i=1}^{N} \sum_{j=1}^{n_{i}} \lambda_{i,j} \textbf{v}_{i,j} \\
    & (5.b) \quad  \sum_{i=1}^{N} \sum_{j=1}^{n_{i}} \lambda_{i,j} = 1, \ \ \lambda_{i,j} \in [0, 1] \\
    & (5.c) \quad  \sum_{k=1,...,N}^{k \neq i} \sum_{j=1}^{n_{k}} \lambda_{k,j} \leq \sum_{l=1}^{m} |z_{l} - \Bar{z}_{i,l}|
\end{aligned}
\label{Eqn:MICP_formulation_all}
\end{equation}

The set of constraint in \eqref{Eqn:MICP_formulation_all} enforces \eqref{Eqn:MICP_formulation_one} for all polytopes, as $\sum_{l=1}^{m} |z_{l} - \Bar{z}_{i,l}| = 0$ only when $\textbf{z}=\Bar{\textbf{z}}_{i}$, enforcing that all $\lambda$'s that are not associated with polytope $i$ to be zero. If $\textbf{z} \neq \Bar{\textbf{z}}_{i}$, $\sum_{l=1}^{m} |z_{l} - \Bar{z}_{i,l}| \geq 1$ and constraint (5.c) is looser than constraint (5.b), hence, trivial.

Note that formulation \eqref{Eqn:MICP_formulation_all} works for any convex polytope that can be written as $\textbf{A}_{i}\textbf{x}\leq \textbf{b}_{i}$. In this paper, the polytopes are McCormick envelope constraints which is a special case.
